# Supplementary material for: Cool molecular highly charged ions for precision tests of fundamental physics
Source: arXiv:2203.10333 ancillary file (2022-03-19)
Supplement: Supplementary file 1 [file supplementary_materials.pdf]

# Supplementary Material for

## Cool molecular highly charged ions for precision tests of fundamental physics

Carsten Zülch,<sup>1</sup> Konstantin Gaul,<sup>1,\*</sup> Steffen M. Giesen,<sup>1</sup> Ronald F. Garcia Ruiz,<sup>2</sup> and Robert Berger<sup>1,†</sup>

<sup>1</sup>*Fachbereich Chemie, Philipps-Universität Marburg, Hans-Meerwein-Straße 4, 35032 Marburg, Germany*

<sup>2</sup>*Massachusetts Institute of Technology, Cambridge, MA 02139, USA*

(Dated: March 19, 2022)

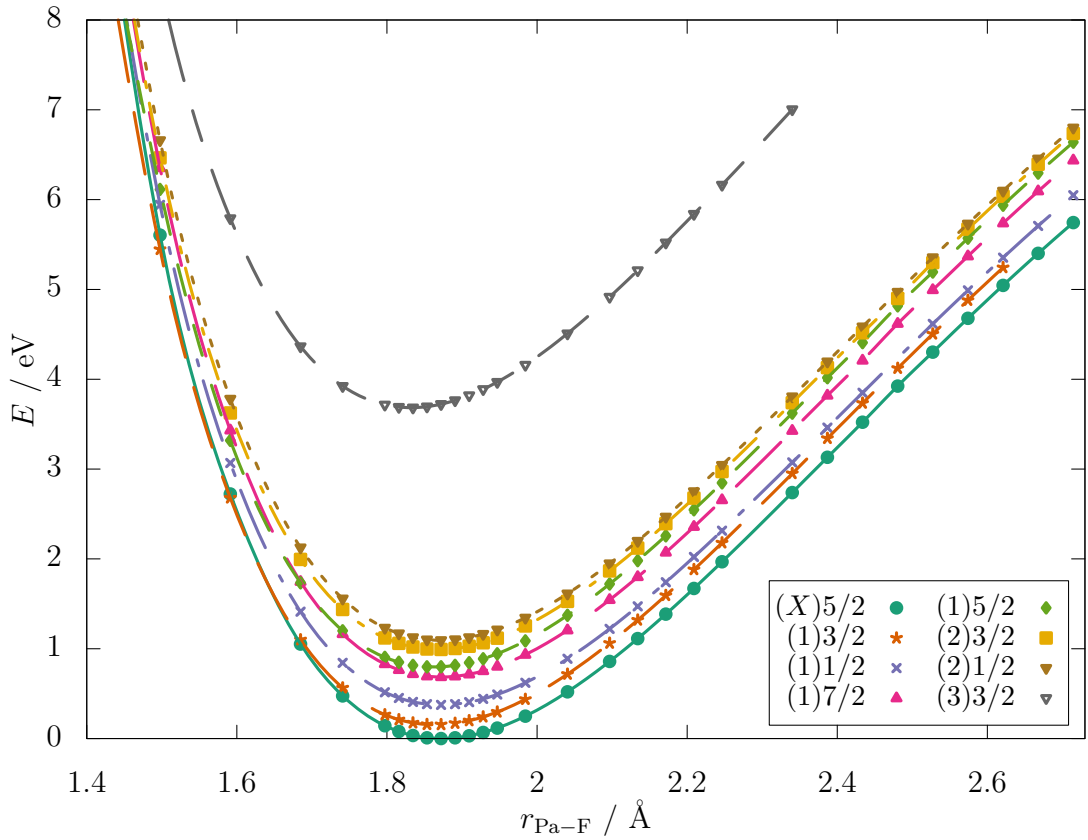

FIG. S1.  **$\text{PaF}^{3+}$  potential energy curves computed on the level of ZORA-cGHE.** The eight energetically lowest electronic states relative to the ground state are depicted. Lines between the points are shown to guide the eye.

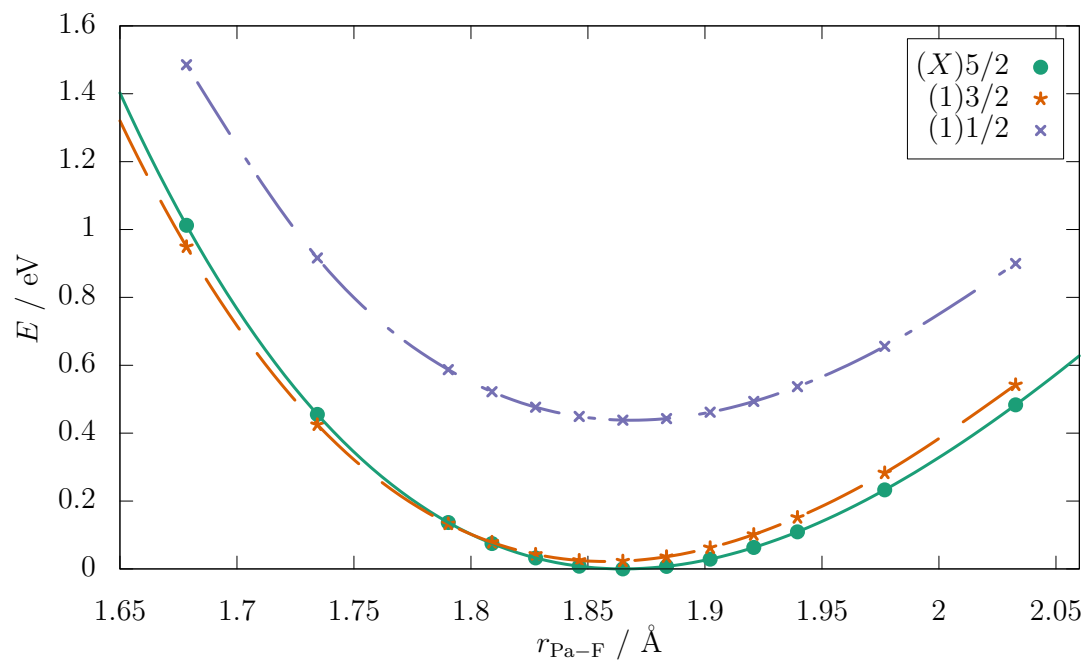

FIG. S2.  $\text{PaF}^{3+}$  potential energy curves computed on the level of ZORA-cGKS-PBE0. The three energetically lowest electronic states relative to the ground state are depicted. Lines between the points are shown to guide the eye.

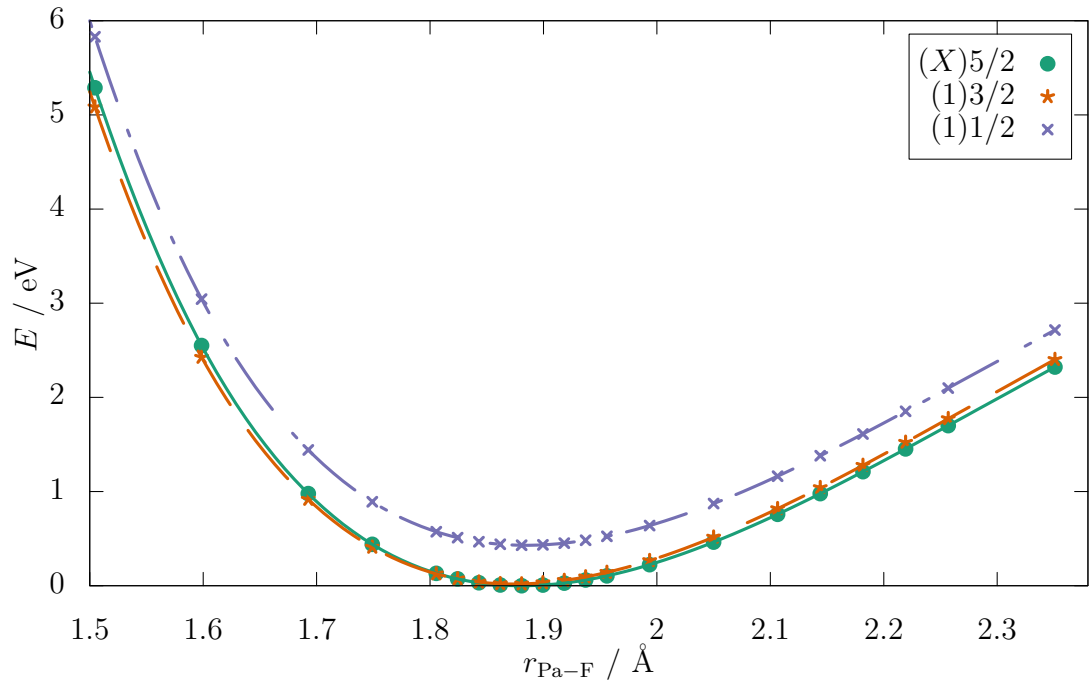

FIG. S3.  $\text{PaF}^{3+}$  potential energy curves computed on the level of ZORA-cGKS-B3LYP. The three energetically lowest electronic states relative to the ground state are depicted. Lines between the points are shown to guide the eye.

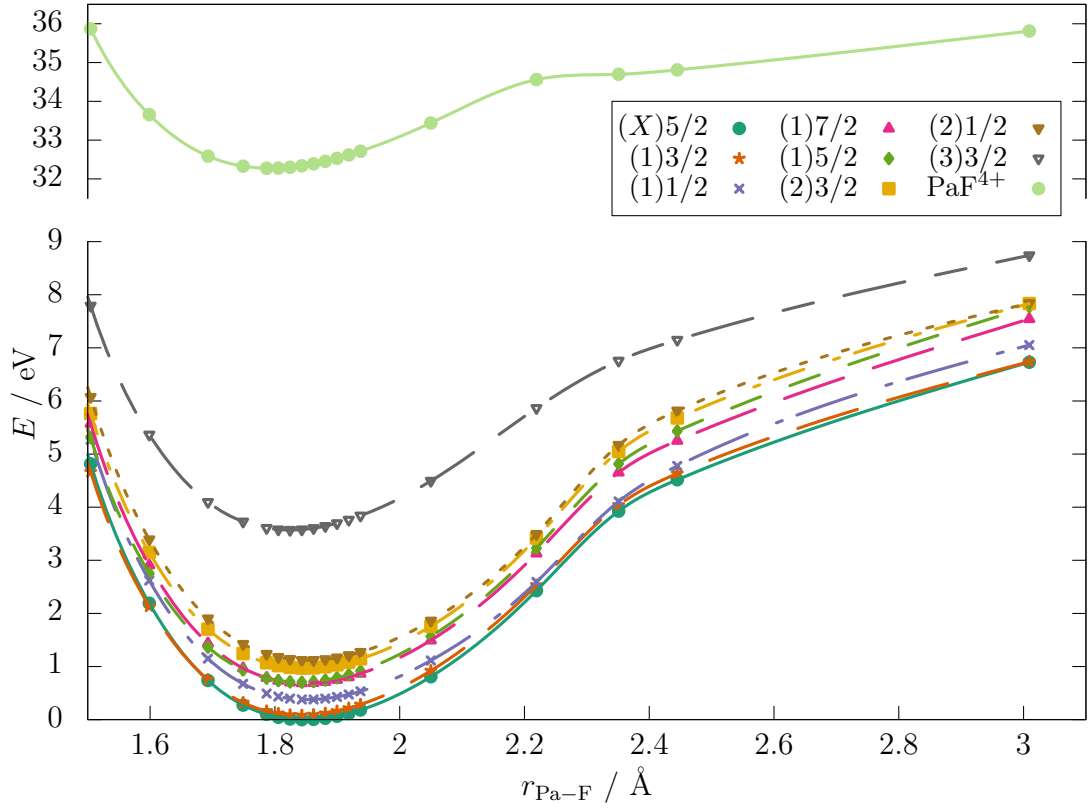

FIG. S4.  $\text{PaF}^{3+}$  and  $\text{PaF}^{4+}$  potential energy curves computed on the level of DC-FSCCSD/ae3z. The eight energetically lowest electronic states relative to the ground state are depicted for  $\text{PaF}^{3+}$ . Lines between the points are shown to guide the eye. The pronounced change in slope of the potential energy curve of  $\text{PaF}^{4+}$ , apparent at an internuclear distance of about 2.2 Å, is understood as an indication for an avoided crossing of electronic states with different character as indicated in Fig. 1 of the main text. In a Fock-space coupled cluster approach, this can also induce a change in slope for the potentials of  $\text{PaF}^{3+}$ .

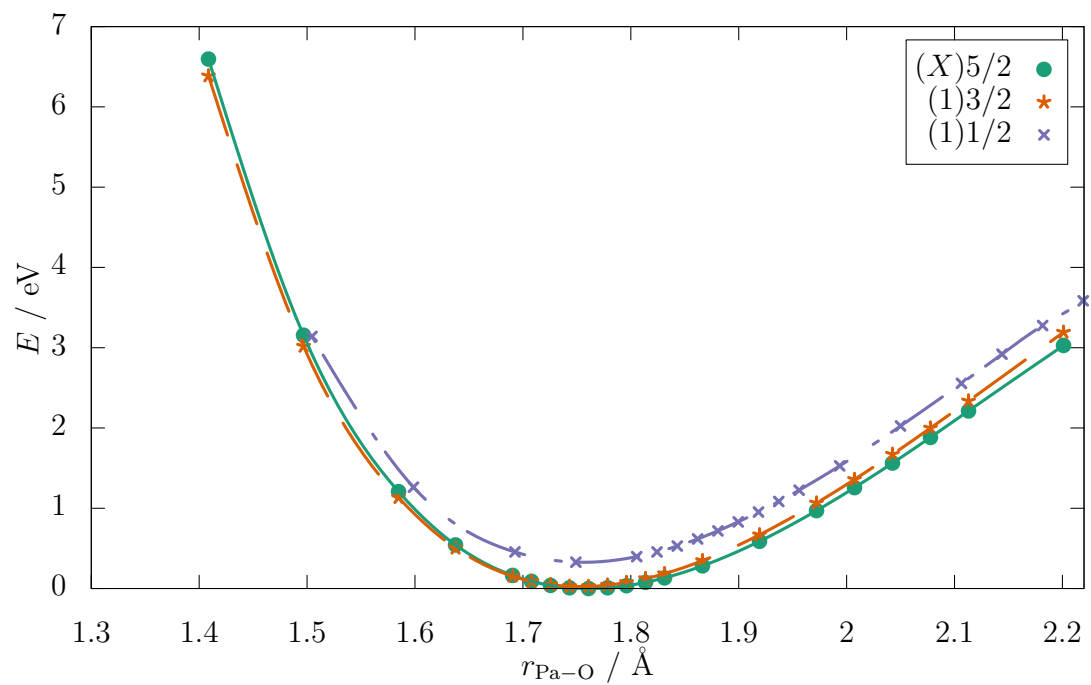

FIG. S5.  $\text{PaO}^{2+}$  potential energy curves computed on the level of ZORA-cGKS-B3LYP. The three energetically lowest electronic states relative to the ground state are depicted. Lines between the points are shown to guide the eye.

TABLE S1. Energies relative to the ground state at equilibrium bond length of  $\text{PaF}^{3+}$  as a function of the Pa-F bond length calculated on the level of ZORA-cGHE.

| $r/\text{\AA}$ | $\Delta E/\text{cm}^{-1}$ |           |           |           |           |           |           |            |
|----------------|---------------------------|-----------|-----------|-----------|-----------|-----------|-----------|------------|
|                | (X)5/2                    | (1)3/2    | (1)1/2    | (1)7/2    | (1)5/2    | (2)3/2    | (2)1/2    | (3)3/2     |
| 1.40           | 86 492.53                 | 80 399.11 | 85 581.13 | 89 434.73 | 82 593.01 | 89 459.12 | 53 714.58 | 103 623.79 |
| 1.50           | 45 205.83                 | 43 920.96 | 47 917.31 | 51 230.50 | 49 311.86 | 52 146.84 | 30 495.43 | 67 924.69  |
| 1.59           | 21 960.47                 | 21 605.98 | 24 744.47 | 27 676.56 | 26 766.89 | 29 239.46 | 17 145.35 | 46 709.21  |
| 1.68           | 8486.04                   | 8867.05   | 11 392.77 | 14 078.55 | 13 984.99 | 16 088.81 | 12 559.66 | 35 208.55  |
| 1.74           | 3831.62                   | 4550.03   | 6795.72   | 9388.41   | 9678.53   | 11 590.06 | 9935.00   | 31 645.58  |
| 1.80           | 1153.80                   | 2140.50   | 4156.18   | 6690.27   | 7291.66   | 9036.16   | 9426.56   | 29 973.81  |
| 1.82           | 631.62                    | 1694.11   | 3642.40   | 6163.69   | 6854.36   | 8548.54   | 9079.69   | 29 767.22  |
| 1.83           | 273.03                    | 1405.11   | 3290.04   | 5801.63   | 6574.93   | 8221.31   | 8882.53   | 29 714.27  |
| 1.85           | 66.20                     | 1262.03   | 3087.36   | 5592.11   | 6441.80   | 8042.78   | 8824.00   | 29 803.15  |
| 1.87           | 0.00                      | 1254.13   | 3023.31   | 5523.92   | 6444.09   | 8001.95   | 8893.70   | 30 022.80  |
| 1.89           | 63.97                     | 1371.27   | 3087.50   | 5586.50   | 6571.62   | 8088.50   | 9081.83   | 30 362.84  |
| 1.91           | 248.28                    | 1603.96   | 3270.16   | 5769.92   | 6814.80   | 8292.75   | 9379.21   | 30 813.56  |
| 1.93           | 543.65                    | 1943.24   | 3562.15   | 6064.86   | 7164.65   | 8605.56   | 9777.22   | 31 365.80  |
| 1.95           | 941.38                    | 2380.74   | 3954.85   | 6462.54   | 7612.70   | 9018.39   | 10 843.27 | 32 011.03  |
| 1.98           | 2011.74                   | 3519.26   | 5010.62   | 7533.75   | 8772.25   | 10 112.44 | 13 010.70 | 33 548.77  |
| 2.04           | 4196.20                   | 5781.52   | 7163.48   | 9721.25   | 11 065.41 | 12 318.26 | 15 712.64 | 36 367.68  |
| 2.10           | 6925.26                   | 8564.46   | 9851.84   | 12 454.68 | 13 878.17 | 15 054.77 | 17 741.62 | 39 654.64  |
| 2.13           | 8976.47                   | 10 640.91 | 11 872.24 | 14 509.23 | 15 973.77 | 17 104.76 | 19 911.95 | 42 036.65  |
| 2.17           | 11 171.34                 | 12 854.01 | 14 034.27 | 16 707.61 | 18 205.43 | 19 294.48 | 22 193.76 | 44 529.61  |
| 2.21           | 13 479.22                 | 15 174.21 | 16 307.97 | 19 019.03 | 20 543.58 | 21 594.02 | 24 561.09 | 47 101.31  |
| 2.25           | 15 873.38                 | 17 575.82 | 18 667.29 | 21 416.62 | 22 962.48 | 23 977.33 | 30 713.07 | 49 715.83  |
| 2.34           | 22 090.57                 | 23 796.22 | 24 798.94 | 27 640.81 | 29 222.53 | 30 160.36 | 33 849.19 | 56 494.73  |
| 2.39           | 25 254.31                 | 26 957.43 | 27 924.20 | 30 805.49 | 32 399.36 | 33 304.89 | 36 988.04 | —          |
| 2.43           | 28 405.80                 | 30 115.28 | 31 050.97 | 33 944.23 | 35 555.26 | 36 437.53 | 40 101.32 | —          |
| 2.48           | 31 646.83                 | 33 247.49 | —         | 37 248.94 | 38 856.81 | 39 522.33 | 43 201.39 | —          |
| 2.53           | 34 700.65                 | 36 332.64 | 37 233.85 | 40 283.03 | 41 890.66 | 42 738.21 | 46 226.31 | —          |
| 2.57           | 37 733.58                 | 39 353.13 | 40 243.88 | 43 313.11 | 44 926.54 | 45 748.96 | 49 185.40 | —          |
| 2.62           | 40 694.86                 | 42 290.64 | 43 182.70 | 46 274.10 | 47 893.94 | 48 701.79 | 52 063.25 | —          |
| 2.67           | 43 567.09                 | —         | 46 035.42 | 49 146.73 | 50 774.13 | 51 571.81 | 54 848.09 | —          |
| 2.71           | 46 336.10                 | —         | 48 787.54 | 51 917.64 | 53 554.37 | 54 340.34 | 57 523.55 | —          |

TABLE S2. Energies relative to the ground state at equilibrium bond length of  $\text{PaF}^{3+}$  and  $\text{PaF}^{4+}$  as a function of the Pa–F internuclear distance calculated on the level of ZORA-cGKS-PBE0.

| $r/\text{\AA}$ | $\Delta E/\text{cm}^{-1}$ |            |           |                                |
|----------------|---------------------------|------------|-----------|--------------------------------|
|                | (X)5/2                    | (1)3/2     | (1)1/2    | $\text{PaF}^{4+}(\text{X})0_+$ |
| 1.31           | 139 385.33                | 136 559.76 | —         | 125 311.11                     |
| 1.40           | 80 941.94                 | 78 568.69  | —         | 68 934.53                      |
| 1.49           | 44 024.40                 | 42 296.61  | —         | 34 742.98                      |
| 1.59           | 21 261.86                 | 20 198.66  | —         | 14 883.65                      |
| 1.68           | 8165.02                   | 7655.99    | 11 982.51 | 4495.32                        |
| 1.73           | 3672.87                   | 3426.84    | 7390.15   | 1438.66                        |
| 1.79           | 1102.65                   | 1070.07    | 4735.68   | 124.25                         |
| 1.81           | 603.43                    | 631.95     | 4210.78   | 0.00                           |
| 1.83           | 261.08                    | 346.16     | 3843.72   | 9.81                           |
| 1.85           | 63.67                     | 200.97     | 3622.46   | 141.22                         |
| 1.86           | 0.00                      | 185.46     | 3535.74   | 382.57                         |
| 1.88           | 59.51                     | 289.32     | 3572.92   | 722.92                         |
| 1.90           | 232.29                    | 502.90     | 3724.07   | 1152.03                        |
| 1.92           | 509.04                    | 817.16     | 3979.87   | 1660.30                        |
| 1.94           | 881.00                    | 1223.57    | 4331.57   | 2238.76                        |
| 1.98           | 1878.25                   | 2281.46    | 5290.35   | 3573.16                        |
| 2.03           | 3898.76                   | 4375.47    | 7258.75   | 5908.21                        |
| 2.09           | 6398.27                   | —          | —         | 8491.43                        |
| 2.13           | 8259.61                   | —          | —         | 10 279.20                      |
| 2.16           | 10 234.76                 | —          | —         | 12 073.18                      |
| 2.20           | 12 292.39                 | —          | —         | 13 827.45                      |
| 2.24           | 14 404.70                 | —          | —         | 15 480.06                      |
| 2.33           | 19 754.58                 | —          | —         | —                              |

TABLE S3. Energies relative to the ground state at equilibrium bond length of  $\text{PaF}^{3+}$  as a function of the Pa–F internuclear distance calculated on the level of ZORA-cGKS-B3LYP.

| $r/\text{\AA}$ | $\Delta E/\text{cm}^{-1}$ |           |           |
|----------------|---------------------------|-----------|-----------|
|                | (X)5/2                    | (1)3/2    | (1)1/2    |
| 1.50           | 42 649.46                 | 41 004.92 | 47 020.62 |
| 1.60           | 20 572.06                 | 19 562.84 | 24 546.83 |
| 1.69           | 7887.67                   | 7397.23   | 11 632.85 |
| 1.75           | 3544.58                   | 3298.08   | 7190.11   |
| 1.81           | 1063.26                   | 1014.00   | 4624.83   |
| 1.82           | 581.79                    | 588.96    | 4117.91   |
| 1.84           | 251.77                    | 311.12    | 3763.46   |
| 1.86           | 61.51                     | 169.05    | 3549.75   |
| 1.88           | 0.00                      | 152.06    | 3465.73   |
| 1.90           | 57.06                     | 250.09    | 3501.07   |
| 1.92           | 222.91                    | 453.72    | 3646.07   |
| 1.94           | 488.48                    | 754.09    | 3891.62   |
| 1.96           | 845.24                    | 1142.91   | 4229.20   |
| 1.99           | 1800.81                   | 2155.25   | 5148.94   |
| 2.05           | 3733.39                   | 4157.69   | 7034.56   |
| 2.11           | 6118.38                   | 6598.61   | 9381.55   |
| 2.14           | 7890.47                   | 8401.91   | 11 133.97 |
| 2.18           | 9767.11                   | 10 307.57 | 12 995.53 |
| 2.22           | 11 717.70                 | 12 284.67 | 14 936.22 |
| 2.26           | 13 714.88                 | 14 307.48 | 16 928.42 |
| 2.35           | 18 733.42                 | 19 378.75 | 21 900.09 |

TABLE S4. Energies relative to the ground state at equilibrium bond length of  $\text{PaF}^{3+}$  as a function of the Pa–F internuclear distance calculated on the level of DC-FSCSD/ANO-RCC.

| $r/\text{\AA}$ | $\Delta E/\text{cm}^{-1}$ |           |           |           |           |           |           |           |
|----------------|---------------------------|-----------|-----------|-----------|-----------|-----------|-----------|-----------|
|                | (X)5/2                    | (1)3/2    | (1)1/2    | (1)7/2    | (1)5/2    | (2)3/2    | (2)1/2    | (3)3/2    |
| 1.60           | 17 660.08                 | 17 150.88 | 20 986.36 | 23 448.98 | 22 154.66 | 25 283.34 | 27 193.78 | 42 908.91 |
| 1.69           | 5929.76                   | 6009.44   | 9146.43   | 11 570.81 | 10 977.82 | 13 661.97 | 15 220.45 | 32 671.80 |
| 1.79           | 782.39                    | 1263.57   | 3871.49   | 6356.03   | 6262.89   | 8566.38   | 9870.45   | 28 751.08 |
| 1.82           | 99.44                     | 696.29    | 3125.66   | 5657.50   | 5716.38   | 7885.99   | 9105.82   | 28 466.94 |
| 1.84           | 0.00                      | 646.37    | 2991.77   | 5551.86   | 5677.99   | 7784.21   | 8964.65   | 28 545.69 |
| 1.85           | 5.84                      | 675.03    | 2979.58   | 5554.93   | 5712.66   | 7788.02   | 8949.37   | 28 635.18 |
| 1.86           | 46.97                     | 737.72    | 3002.12   | 5593.48   | 5781.54   | 7826.58   | 8969.18   | 28 756.28 |
| 1.87           | 122.12                    | 833.23    | 3058.13   | 5666.26   | 5883.39   | 7898.63   | 9022.83   | 28 907.71 |
| 1.88           | 230.10                    | 960.39    | 3146.37   | 5772.03   | 6017.03   | 8002.99   | 9109.11   | 29 088.19 |
| 1.89           | 369.73                    | 1118.05   | 3265.66   | 5909.62   | 6181.34   | 8138.51   | 9226.83   | 29 296.55 |
| 1.90           | 539.88                    | 1305.12   | 3414.85   | 6077.90   | 6375.22   | 8304.08   | 9374.89   | 29 531.62 |
| 1.91           | 739.48                    | 1520.56   | 3592.85   | 6275.76   | 6597.62   | 8498.65   | 9552.19   | 29 792.27 |
| 1.94           | 1504.73                   | 2327.11   | 4289.15   | 7036.62   | 7426.08   | 9246.33   | 10 249.38 | 30 717.17 |
| 1.97           | 2878.52                   | 3742.41   | 5560.14   | 8406.29   | 8873.30   | 10 592.03 | 11 530.07 | 32 247.42 |
| 2.07           | 7776.10                   | 8682.71   | 10 123.28 | 13 303.29 | 13 914.84 | 15 414.88 | 16 194.65 | 37 228.86 |
| 2.26           | 24 245.93                 | 25 069.88 | 25 155.70 | 29 981.68 | 30 921.81 | 32 578.83 | 33 263.23 | 50 169.94 |
| 2.44           | 36 540.21                 | 37 839.99 | 39 147.25 | 42 544.85 | 44 215.65 | 44 702.07 | 45 284.66 | 59 208.57 |

TABLE S5. Energies relative to the ground state at equilibrium bond length of  $\text{PaF}^{3+}$  as a function of the Pa–F internuclear distance calculated on the level of DC-FSCSD/ae3z. The  $\text{PaF}^{4+}$  energies are computed for the ground state.

| $r/\text{\AA}$ | $\Delta E/\text{cm}^{-1}$ |           |           |           |           |           |           |           |                                |
|----------------|---------------------------|-----------|-----------|-----------|-----------|-----------|-----------|-----------|--------------------------------|
|                | (X)5/2                    | (1)3/2    | (1)1/2    | (1)7/2    | (1)5/2    | (2)3/2    | (2)1/2    | (3)3/2    | $\text{PaF}^{4+}(\text{X})0_+$ |
| 1.41           | 73 712.98                 | 71 710.71 | 77 894.44 | 80 615.71 | 77 565.65 | 81 539.39 | 84 822.55 | 96 361.97 | 321 033.99                     |
| 1.50           | 38 836.05                 | 37 612.32 | 42 496.65 | 44 944.48 | 42 805.16 | 46 487.12 | 48 982.17 | 62 843.16 | 289 303.60                     |
| 1.60           | 17 665.54                 | 17 194.97 | 21 120.98 | 23 444.50 | 22 183.43 | 25 387.88 | 27 354.89 | 43 271.19 | 271 467.49                     |
| 1.69           | 5943.88                   | 6049.52   | 9263.64   | 11 580.50 | 11 006.96 | 13 750.28 | 15 353.46 | 33 031.76 | 262 843.26                     |
| 1.75           | 2209.92                   | 2570.54   | 5443.22   | 7801.67   | 7543.23   | 10 042.11 | 11 477.57 | 30 062.16 | 260 753.69                     |
| 1.79           | 795.19                    | 1292.19   | 3964.22   | 6366.54   | 6282.22   | 8632.35   | 9970.72   | 29 093.42 | 260 324.21                     |
| 1.81           | 365.97                    | 922.05    | 3500.47   | 5929.19   | 5922.25   | 8202.04   | 9495.41   | 28 866.75 | 260 351.07                     |
| 1.82           | 104.87                    | 714.38    | 3203.08   | 5661.07   | 5725.56   | 7937.56   | 9187.96   | 28 794.06 | 260 520.33                     |
| 1.84           | 0.00                      | 657.64    | 3060.09   | 5550.16   | 5680.52   | 7827.13   | 9036.38   | 28 863.14 | 260 819.15                     |
| 1.86           | 40.35                     | 741.06    | 3060.06   | 5585.35   | 5776.43   | 7860.02   | 9029.95   | 29 062.64 | 261 235.52                     |
| 1.88           | 215.65                    | 954.74    | 3193.53   | 5756.13   | 6002.98   | 8025.58   | 9157.15   | 29 382.06 | 261 758.33                     |
| 1.90           | 516.43                    | 1289.41   | 3449.95   | 6053.08   | 6351.27   | 8315.00   | 9409.68   | 29 811.55 | 262 377.06                     |
| 1.92           | 933.86                    | 1736.50   | 3820.65   | 6467.25   | 6812.63   | 8719.45   | 9778.30   | 30 342.06 | 263 082.00                     |
| 1.94           | 1459.85                   | 2288.13   | 4297.29   | 6990.50   | 7379.23   | 9231.00   | 10 254.94 | 30 965.14 | 263 864.01                     |
| 2.05           | 6517.54                   | 7424.15   | 8984.35   | 12 042.59 | 12 627.02 | 14 188.24 | 15 013.19 | 36 247.34 | 269 729.34                     |
| 2.22           | 19 592.38                 | 20 412.12 | 20 901.67 | 25 247.15 | 26 053.33 | 27 571.59 | 28 175.59 | 47 302.55 | 278 758.47                     |
| 2.35           | 31 664.28                 | 32 563.31 | 33 128.14 | 37 543.31 | 38 839.32 | 40 736.74 | 41 696.21 | 54 495.69 | 279 853.32                     |
| 2.44           | 36 428.10                 | 37 371.17 | 38 527.70 | 42 359.89 | 43 839.29 | 45 810.21 | 46 910.95 | 57 662.75 | 280 769.62                     |
| 3.01           | 54 277.64                 | 54 362.77 | 56 885.68 | 60 846.92 | 62 711.33 | 63 187.59 | 63 227.08 | 70 499.26 | 288 848.81                     |

TABLE S6. **Energies of the ground state (X)5/2 and first excited state (1)3/2 relative to the ground state at equilibrium bond length of  $\text{PaO}^{2+}$  as a function of the Pa–O internuclear distance calculated on the level of ZORA-cGKS-B3LYP.**

| $r/\text{\AA}$ | $\Delta E/\text{cm}^{-1}$ |           |
|----------------|---------------------------|-----------|
|                | (X)5/2                    | (1)3/2    |
| 1.41           | 53 199.02                 | 51 511.85 |
| 1.50           | 25 455.32                 | 24 341.34 |
| 1.58           | 9736.75                   | 9146.25   |
| 1.64           | 4379.57                   | 4063.94   |
| 1.69           | 1316.38                   | 1241.59   |
| 1.71           | 720.73                    | 721.86    |
| 1.73           | 311.92                    | 383.56    |
| 1.74           | 76.00                     | 214.83    |
| 1.76           | 0.00                      | 202.77    |
| 1.78           | 71.77                     | 335.37    |
| 1.80           | 279.99                    | 601.38    |
| 1.81           | 614.03                    | 990.31    |
| 1.83           | 1063.93                   | 1492.34   |
| 1.87           | 2274.63                   | 2799.40   |
| 1.92           | 4744.22                   | 5395.84   |
| 1.97           | 7825.46                   | 8585.80   |
| 2.01           | 10 136.73                 | 10 961.31 |
| 2.04           | 12 603.33                 | 13 487.08 |
| 2.08           | 15 186.19                 | 16 125.98 |
| 2.11           | 17 846.93                 | 18 843.55 |
| 2.20           | 24 422.31                 | 25 748.26 |

TABLE S7.  
**Energies of the  
second excited  
state  $(1)1/2$   
relative to the  
ground state at  
equilibrium bond  
length of  $\text{PaO}^{2+}$   
as a function of  
the Pa–O inter-  
nuclear distance  
calculated on the  
level of ZORA-  
cGKS-B3LYP.**

| $r/\text{\AA}$ | $\Delta E/\text{cm}^{-1}$ |
|----------------|---------------------------|
| 1.50           | 25 333.85                 |
| 1.60           | 10 181.25                 |
| 1.69           | 3671.92                   |
| 1.75           | 2646.14                   |
| 1.81           | 3202.82                   |
| 1.82           | 3675.25                   |
| 1.84           | 4271.11                   |
| 1.86           | 4979.60                   |
| 1.88           | 5790.62                   |
| 1.90           | 6694.75                   |
| 1.92           | 7683.16                   |
| 1.94           | 8747.60                   |
| 1.96           | 9880.33                   |
| 1.99           | 12 322.08                 |
| 2.05           | 16 329.64                 |
| 2.11           | 20 615.25                 |
| 2.14           | 23 552.20                 |
| 2.18           | 26 426.12                 |
| 2.22           | 28 909.75                 |
| 2.26           | 32 586.00                 |

TABLE S8. Spectroscopically relevant properties of the three energetically lowest electronic states of  $\text{PaO}^{2+}$ . Equilibrium bond length  $r_e$ , harmonic vibrational wavenumber  $\tilde{\omega}_e$  and excitation wavenumber  $\tilde{T}_e$  estimated as vertical excitation energies are shown at the level of ZORA-cGKS-B3LYP using the ANO-RCC-VDZP basis set [1] for oxygen and the even tempered basis set for Pa also used in the  $\text{PaF}^{3+}$  calculations. The projection of the electronic orbital angular momentum quantum number on the molecular axis  $\Lambda$ , the squared transition dipole moment  $|\vec{\mu}_T|^2$ , hyperfine coupling constant along the molecular axis  $A_{\parallel}$ , electronic structure enhancement of the nuclear Schiff moment  $W_S$  are shown. For  $A_{\parallel} \mu(^{231}\text{Pa}) \simeq 2.01\mu_N$  and  $I = 3/2$  [2] was used.

| State  | $r_e / \text{\AA}$ | $\tilde{\omega}_e / \text{cm}^{-1}$ | $\tilde{T}_e / \text{cm}^{-1}$ | $\Lambda$ | $ \vec{\mu}_T ^2 / e^2 a_0^2$ | $A_{\parallel} / \text{MHz}$ | $W_S / \frac{e}{4\pi\epsilon_0 a_0^4}$ |
|--------|--------------------|-------------------------------------|--------------------------------|-----------|-------------------------------|------------------------------|----------------------------------------|
| (X)5/2 | 1.77               | 987                                 | —                              | 2.8       |                               | −1033                        | −67 152                                |
| (1)3/2 | 1.76               | 977                                 | 203                            | 1.9       | $3.72 \times 10^{-2}$         | −1015                        | −59 769                                |
| (1)1/2 | 1.77               | 987                                 | 2645                           | 0.7       | $4.09 \times 10^{-10}$        | −1443                        | −53 375                                |

\* konstantin.gaul@staff.uni-marburg.de; kongaul@web.de

† robert.berger@uni-marburg.de

- [1] Roos, B. O., Lindh, R., Malmqvist, P., Veryazov, V. & Widmark, P. O. Main Group Atoms and Dimers Studied with a New Relativistic ANO Basis Set. *J. Phys. Chem. A* **108**, 2851–2858 (2004).
- [2] Axe, J. D., Stapleton, H. J. & Jeffries, C. D. Paramagnetic resonance hyperfine structure of tetravalent  $\text{Pa}^{231}$  in  $\text{Cs}_2\text{ZrCl}_6$ . *Phys. Rev.* **121**, 1630–1637 (1961). URL <https://link.aps.org/doi/10.1103/PhysRev.121.1630>.
